# Supplementary material for: SonicChain: A Wait-free, Pseudo-Static Approach Toward Concurrency in Blockchains
Source: arXiv:2102.09073 source file (2021-02-06)
Supplement: Supplementary file 1 [file appendix.tex]

\chapter*{Appendix}
